# Supplementary material for: Density-Functional Theory of Thermoelectric Phenomena
Source: arXiv:1308.2311 source file (2014-05-15)
Supplement: Supplementary file 1 [file ThermalDFT-SupplementalMaterial.pdf]

# Density Functional Theory of Thermoelectric Phenomena

***Supplemental Material***

F. G. Eich,[1,*] M. Di Ventra,[2] and G. Vignale[1]

[1] *Department of Physics, University of Missouri-Columbia, Columbia, Missouri 65211*

[2] *University of California, San Diego, La Jolla, CA 92093*

(Dated: April 2, 2014)

## KOHN-SHAM CONSTRUCTION

Let us first recall the decompositions of the universal functionals of the interacting and the KS system,

$$A[n,h] \equiv A^{\mathrm{eq}}[n] + \int_{\mathcal{C}} \int \mathrm{d}^3 r \; \bar{h}[n,h](\boldsymbol{r},\tau) - \bar{S}[n,h] \; , \tag{1a}$$

$$A_{\mathrm{s}}[n,h_{\mathrm{s}}] \equiv A_{\mathrm{s}}^{\mathrm{eq}}[n] + \int_{\mathcal{C}} \int \mathrm{d}^3 r \; \bar{h}_{\mathrm{s}}[n,h_{\mathrm{s}}](\boldsymbol{r},\tau) - \bar{S}_{\mathrm{s}}[n,h_{\mathrm{s}}] \; . \tag{1b}$$

Now we know that the thermal field of the interacting system is given by

$$\psi(\boldsymbol{r},t) = -\frac{\delta A[n,h]}{\delta h(\boldsymbol{r},t)} = -1 + \frac{\delta \bar{S}[n,h]}{\delta h(\boldsymbol{r},t)} \; , \tag{2}$$

and the thermal field of the KS system by

$$\psi_{\mathrm{s}}(\boldsymbol{r},t) = -\frac{\delta A_{\mathrm{s}}[n,h_{\mathrm{s}}]}{\delta h_{\mathrm{s}}(\boldsymbol{r},t)} = -1 + \frac{\delta \bar{S}_{\mathrm{s}}[n,h_{\mathrm{s}}]}{\delta h_{\mathrm{s}}(\boldsymbol{r},t)} \; . \tag{3}$$

In order to connect the KS thermal field to the interacting thermal field it is important to remember that the energy density arguments differ for the interacting and the KS system. We have to evaluate Eq. (2) at $h = h_{\mathrm{s}} + \mathcal{E}_{\mathrm{Hxc}}[n]$. Since this is just a shift of the energy-density argument for the interacting functional we obtain from Eqs. (2), (3)

$$\psi_{\mathrm{s}}(\boldsymbol{r},t) = \psi(\boldsymbol{r},t) - \frac{\delta \bar{S}_{\mathrm{xc}}[n,h_{\mathrm{s}}]}{\delta h_{\mathrm{s}}(\boldsymbol{r},t)} \; , \tag{4}$$

where we defined

$$\bar{S}_{\mathrm{xc}}[n,h_{\mathrm{s}}] \equiv \bar{S}[n,h_{\mathrm{s}} + \mathcal{E}_{\mathrm{Hxc}}[n]] - \bar{S}_{\mathrm{s}}[n,h_{\mathrm{s}}] \; . \tag{5}$$

Turning to the potential of the interacting system we have

$$\tilde{v}(\boldsymbol{r},t) = -\frac{\delta A[n,h]}{\delta n(\boldsymbol{r},t)} = -\frac{\delta A^{\mathrm{eq}}[n]}{\delta n(\boldsymbol{r},t)} - \int \mathrm{d}^3 r' \; \frac{\delta \bar{h}[n,h](\boldsymbol{r}',t)}{\delta n(\boldsymbol{r},t)} + \frac{\delta \bar{S}[n,h]}{\delta n(\boldsymbol{r},t)} \; , \tag{6}$$

and similarly for the KS system

$$\tilde{v}_{\mathrm{s}}(\boldsymbol{r},t) = -\frac{\delta A_{\mathrm{s}}[n,h_{\mathrm{s}}]}{\delta n(\boldsymbol{r},t)} = -\frac{\delta A_{\mathrm{s}}^{\mathrm{eq}}[n]}{\delta n(\boldsymbol{r},t)} - \int \mathrm{d}^3 r' \; \frac{\delta \bar{h}_{\mathrm{s}}[n,h_{\mathrm{s}}](\boldsymbol{r}',t)}{\delta n(\boldsymbol{r},t)} + \frac{\delta \bar{S}_{\mathrm{s}}[n,h_{\mathrm{s}}]}{\delta n(\boldsymbol{r},t)} \; . \tag{7}$$

Again we evaluate the interacting functionals at the energy density $h = h_{\mathrm{s}} + \mathcal{E}_{\mathrm{Hxc}}[n]$. Some care has to be taken in writing the functional derivatives w.r.t. $n$, since the shift in the energy density argument *depends* on $n$. For example we have

$$\left.\frac{\delta \bar{S}[n,h]}{\delta n(\boldsymbol{r},t)}\right|_{h=h_{\mathrm{s}}+\mathcal{E}_{\mathrm{Hxc}}} = \frac{\delta \bar{S}[n,h_{\mathrm{s}}+\mathcal{E}_{\mathrm{Hxc}}[n]]}{\delta n(\boldsymbol{r},t)} - \int \mathrm{d}^3 r' \; \frac{\delta \bar{S}[n,h_{\mathrm{s}}+\mathcal{E}_{\mathrm{Hxc}}]}{\delta h_{\mathrm{s}}(\boldsymbol{r}',t)} \frac{\delta \mathcal{E}_{\mathrm{Hxc}}[n](\boldsymbol{r}',t)}{\delta n(\boldsymbol{r},t)} \; . \tag{8}$$

The second term on the r.h.s. is needed as counter term since we are shifting the energy argument by an $n$-dependent quantity $\mathcal{E}_{\mathrm{Hxc}}[n]$ *before* evaluating the functional derivative w.r.t. $n$. A similar counter term has to be added when

shifting the energy argument of $\bar{h}[n,h]$ inside the functional derivative. Using $1+\psi = \frac{\delta \bar{S}[n,h_\mathrm{s}+\mathcal{E}_\mathrm{Hxc}]}{\delta h_\mathrm{s}}$ [cf. Eq. (2)] and the definition $\bar{h}[n,h] = h - h^\mathrm{eq}[n]$ we rewrite Eq. (6) as follows:

$$\tilde{v}(\boldsymbol{r},t) = -\frac{\delta A^\mathrm{eq}[n]}{\delta n(\boldsymbol{r},t)} + \int \mathrm{d}^3r' \, \frac{\delta h^\mathrm{eq}[n](\boldsymbol{r}',t)}{\delta n(\boldsymbol{r},t)} + \frac{\delta \bar{S}[n,h_\mathrm{s}+\mathcal{E}_\mathrm{Hxc}[n]]}{\delta n(\boldsymbol{r},t)} - \int \mathrm{d}^3r' \, [1+\psi(\boldsymbol{r}',t)] \frac{\delta \mathcal{E}_\mathrm{Hxc}[n](\boldsymbol{r}',t)}{\delta n(\boldsymbol{r},t)} \ . \tag{9}$$

A similar expression can be written for the Kohn-Sham potential from Eq. (7):

$$\tilde{v}_\mathrm{s}(\boldsymbol{r},t) = -\frac{\delta A_\mathrm{s}^\mathrm{eq}[n]}{\delta n(\boldsymbol{r},t)} + \int \mathrm{d}^3r' \, \frac{\delta h_\mathrm{s}^\mathrm{eq}[n](\boldsymbol{r}',t)}{\delta n(\boldsymbol{r},t)} + \frac{\delta \bar{S}_\mathrm{s}[n,h_\mathrm{s}]}{\delta n(\boldsymbol{r},t)} \ . \tag{10}$$

Now we can connect the KS potential to the interacting potential via

$$\tilde{v}_\mathrm{s}(\boldsymbol{r},t) = \tilde{v}(\boldsymbol{r},t) + \frac{\delta\left(A^\mathrm{eq}[n] - A_\mathrm{s}^\mathrm{eq}[n]\right)}{\delta n(\boldsymbol{r},t)} + \int \mathrm{d}^3r' \, \psi(\boldsymbol{r}',t) \frac{\delta \mathcal{E}_\mathrm{Hxc}[n](\boldsymbol{r}',t)}{\delta n(\boldsymbol{r},t)} - \frac{\delta \bar{S}_\mathrm{xc}[n,h_\mathrm{s}]}{\delta n(\boldsymbol{r},t)} \ , \tag{11}$$

where use has been made of the identity $h^\mathrm{eq}[n] - h_\mathrm{s}^\mathrm{eq}[n] = \mathcal{E}_\mathrm{Hxc}[n]$ and the definition (5) of the xc excess entropy. This establishes the splitting of the KS potential:

$$\tilde{v}_\mathrm{s}[n,h_\mathrm{s}](\boldsymbol{r},t) = \tilde{v}(\boldsymbol{r},t) + \tilde{v}_\mathrm{Hxc}^\mathrm{eq}[n(t)](\boldsymbol{r}) + \bar{v}_\mathrm{xc}[n,h_\mathrm{s}](\boldsymbol{r},t) \ , \tag{12a}$$

$$\tilde{v}_\mathrm{Hxc}^\mathrm{eq}[n(t)](\boldsymbol{r}) = v_\mathrm{Hxc}^\mathrm{eq}[n(t)](\boldsymbol{r}) + \int \mathrm{d}^3r' \, \psi(\boldsymbol{r}',t) \frac{\delta \mathcal{E}_\mathrm{Hxc}[n(t)](\boldsymbol{r}')}{\delta n(\boldsymbol{r},t)} \ , \tag{12b}$$

$$\bar{v}_\mathrm{xc}[n,h_\mathrm{s}](\boldsymbol{r},t) = -\frac{\delta \bar{S}_\mathrm{xc}[n,h_\mathrm{s}]}{\delta n(\boldsymbol{r},t)} \ , \tag{12c}$$

where we used

$$v_\mathrm{Hxc}^\mathrm{eq}[n(t)](\boldsymbol{r}) = \frac{\delta\left(A^\mathrm{eq}[n] - A_\mathrm{s}^\mathrm{eq}[n]\right)}{\delta n(\boldsymbol{r},t)} = \frac{\delta\left(F^\mathrm{eq}[n(t)] - F_\mathrm{s}^\mathrm{eq}[n(t)]\right)}{\delta n(\boldsymbol{r},t)} \ . \tag{13}$$

## DETAILS OF THE ADIABATIC APPROXIMATION

The adiabatic approximation to the excess entropy reads,

$$\bar{S}^\mathrm{A}[n,h] = \frac{1}{\beta} \int_\mathcal{C} \left(S^\mathrm{qeq}[n(\tau),h(\tau)] - S^\mathrm{eq}[n(\tau)]\right) \ , \tag{14}$$

where we approximated $S[n,h]$ by an instantaneous functional of the density and energy density, i.e., we ignored retardation effects. It can be shown that the instantaneous entropy $S^\mathrm{qeq}[n(\tau),h(\tau)]$ is defined as the maximal entropy under the constraint that the density is fixed to $n(\boldsymbol{r},\tau)$ and the energy density to $h(\boldsymbol{r},\tau)$. Similarly we can define the adiabatic approximation for the excess entropy of the KS system, $\bar{S}_\mathrm{s}^\mathrm{A}[n,h_\mathrm{s}]$, which leads to the definition of the adiabatic xc excess entropy

$$\bar{S}_\mathrm{xc}^\mathrm{A}[n,h_\mathrm{s}] = \bar{S}^\mathrm{A}[n,h_\mathrm{s}+\mathcal{E}_\mathrm{Hxc}[n]] - \bar{S}_\mathrm{s}^\mathrm{A}[n,h_\mathrm{s}] \ . \tag{15}$$

Hence, the adiabatic approximation to $\bar{v}_\mathrm{xc}$ is given by

$$\bar{v}_\mathrm{xc}^\mathrm{A}[n(t),h_\mathrm{s}(t)](\boldsymbol{r}) = -\tfrac{1}{\beta} \frac{\delta S_\mathrm{xc}^\mathrm{A}[n(t),h_\mathrm{s}(t)]}{\delta n(\boldsymbol{r},t)} \ , \tag{16}$$

From Eq. (14) we see that $\bar{v}_\mathrm{xc}^\mathrm{A}$ contains a piece from the difference of $S^\mathrm{eq}[n]$ and $S_\mathrm{s}^\mathrm{eq}[n]$. Comparing this to Eq. (13) and remembering that $F^\mathrm{eq}[n] = \int \mathrm{d}^3r \, h^\mathrm{eq}[n](\boldsymbol{r}) - \frac{1}{\beta} S^\mathrm{eq}[n]$ we can see that $v_\mathrm{Hxc}^\mathrm{eq}$ contains the same piece *but* with a different sign. This suggest to cancel the two opposite contributions and redefine

$$\tilde{v}_\mathrm{Hxc}^\mathrm{eq}[n(t)](\boldsymbol{r}) = v_\mathrm{Hxc}[n(t)](\boldsymbol{r}) + \int \mathrm{d}^3r' \, \psi(\boldsymbol{r}',t) \frac{\delta \mathcal{E}_\mathrm{Hxc}[n(t)](\boldsymbol{r}')}{\delta n(\boldsymbol{r},t)} \ , \tag{17a}$$

$$\bar{S}_\mathrm{xc}^\mathrm{A}[n,h_\mathrm{s}] = \frac{1}{\beta} \left(S^\mathrm{qeq}[n(t),h_\mathrm{s}(t)+\mathcal{E}_\mathrm{Hxc}[n(t)]] - \bar{S}_\mathrm{s}^\mathrm{qeq}[n,h_\mathrm{s}]\right) \ , \tag{17b}$$

where we introduced

$$v_{\mathrm{Hxc}}[n(t)](\boldsymbol{r}) = \frac{\delta}{\delta n(\boldsymbol{r},t)} \int \mathrm{d}^3r' \ \left(h^{\mathrm{eq}}[n(t)](\boldsymbol{r}') - h_{\mathrm{s}}^{\mathrm{eq}}[n(t)](\boldsymbol{r}')\right) = \int \mathrm{d}^3r' \ \frac{\delta \mathcal{E}_{\mathrm{Hxc}}[n(t)](\boldsymbol{r}')}{\delta n(\boldsymbol{r},t)} \equiv \frac{\delta E_{\mathrm{Hxc}}[n(t)]}{\delta n(\boldsymbol{r},t)} \ . \tag{18}$$

Under the assumption that the functional derivative $\frac{\delta \mathcal{E}_{\mathrm{Hxc}}[n(t)](\boldsymbol{r}')}{\delta n(\boldsymbol{r},t)}$ in Eq. (17a) is short-ranged in $|\boldsymbol{r}-\boldsymbol{r}'|$ we get

$$\frac{\delta \mathcal{E}_{\mathrm{Hxc}}[n(t)](\boldsymbol{r}')}{\delta n(\boldsymbol{r},t)} \approx v_{\mathrm{Hxc}}[n(t)](\boldsymbol{r})\delta(\boldsymbol{r}-\boldsymbol{r}') \ , \tag{19}$$

and hence we arrive at the local approximation

$$\tilde{v}_{\mathrm{Hxc}}^{\mathrm{eq}}[n(t)](\boldsymbol{r}) \approx (1+\psi(\boldsymbol{r},t))v_{\mathrm{Hxc}}[n(t)](\boldsymbol{r}) \ . \tag{20}$$

This is the intuitively expected result that the Hxc potential of the ordinary equilibrium theory should be re-scaled to take into account the local "temperature field" $\psi$. Notice, however, that this re-scaling is not and cannot be general, since the exact $v_{\mathrm{Hxc}}(\boldsymbol{r})$ is a non-local functional of the density, which in principle is affected by the entire distribution of $\psi$, not just its value at $\boldsymbol{r}$. It is only in a local-density approximation that the simple re-scaling of Eq. (20) holds.

* eichf@missouri.edu
